# Supplementary material for: Recognizing Entity Types via Properties
Source: arXiv:2304.07910 source file (2023-04-24)
Supplement: Supplementary file 1 [file additional.tex]

\subsubsection{Dealing with trivial samples}
In order to decrease the negative samples and avoid generating unnecessary candidate pairs, we prune the trivial samples which are obvious to be negative. Regarding the above-mentioned two cases, we have:
\begin{itemize}
    \item For schema-level etype recognition, we apply label-based measurements to filter the obviously negative samples. Given two etypes $E_a$ and $E_b$ from a candidate pair, we define the pre-selection factor $PS_s$ as: 
\begin{equation}
PS_s = Ngram(E_a,E_b) + Word2Vec(E_a,E_b)
\label{equ:7}
\end{equation}
    where $Ngram(\cdot)$ and $Word2Vec(\cdot)$ are two similarity measurements which are lexical-based and semantic-based, respectively. Thus, we consider $(E_a,E_b)$ is a obviously negative candidate etype pair if $PS_s$ is greater than the threshold $th$. Experimentally, we find that $th = 0.3$ will lead to better results.
    
    \item For instance-level cases, the obviously negative candidate pair is identified when two entities $I_a$ and $I_b$ have no shared property. Thus, such candidate pairs will be pruned before inputting to the etype recognizer.
\end{itemize}

\noindent
The pre-selection of trivial samples will effectively reduce the run-time for model training. Moreover, such a training strategy will help to decrease the risk of overfitting by alleviating redundant samples and to improve the etype recognition performance.

\section{Similarity metric calculation algorithm}

\begin{algorithm}[htb] 
\caption{Calculating horizontal similarity $Sim_H$ between reference and candidate KGs. $L_H=SimCal_H(f_a,f_b)$} 
\label{alg:1} 
\begin{algorithmic}[1] 
\REQUIRE ~~\\ 
Reference and candidate FCA contexts $f_a$, $f_b$;\\
\ENSURE ~~\\ 
List of all horizontal similarities $L_H$;\\

\STATE $EM = (E_a \times E_b) = EtypeSelector(f_a,f_b)$; \{etypes/entities $E_a, E_b$ from $f_a, f_b$ are assembled as candidate calculation pairs $EM$.\}
\STATE 	$PM = (p_a \times p_b) = PropertyMatcher(f_a,f_b)$; \{$PM$ is formed as a set of aligned property pairs, where $p_a \in f_a$, $p_b \in f_b$.\}
% \STATE  $P(E) = \{p_0...p_n\}$; \{obtain all properties which are used for describing the etype $E$.\}
\FOR {all $(E_j,E_k) \in EM$}
\STATE $sim_H(E_j,E_k) = 0$; \{initialize the value of horizontal similarity $sim_H(E_j,E_k)$.\}
\FOR {all $(p_n,p_m) \in PM$}
\IF {$p_n \in prop(E_j) \wedge p_m \in prop(E_k)$}
\STATE $sim_H(E_j,E_k).add(\frac{HS_A(E_j,p_n)}{|prop(E_j)|} {+} \frac{HS_B(E_k,p_m)}{|prop(E_k)|})$; \{calculate the corresponding specificity $HS$ for the similarity $sim_H(E_j,E_k)$.\}

\ENDIF
\ENDFOR
\STATE $L_H.stack(\frac{1}{2} * sim_H(E_j,E_k))$; 
\{stack the value of horizontal similarity to the list $L_H$.\}

\ENDFOR

\RETURN $L_H$
\end{algorithmic}
\end{algorithm}

We have discussed the processing framework for etype recognition in section 4. Algorithm \ref{alg:1} presents the step-by-step process for calculating our property-based etype similarity metrics, which is a crucial part of the framework. Generally, there will be two input KGs at the beginning, where $KG_{ref}$ provides reference etypes and $KG_{cand}$ is the candidate KG waiting for recognition. After formalizing $KG_{ref}$ and $KG_{cand}$, we assume that the two FCA contexts $f_a$ and $f_b$ are generated correspondingly. $PM$ refers to the property matching pairs which are aligned by the property matcher, $EM$ refers to the candidate etypes/entities pairs for recognition. For every candidate pair in $EM$, we check their correlated properties and update the specificity values to $Sim_H$,  $Sim_V$ and $Sim_I$ when their properties are aligned. After traversing all the candidate pairs, we obtain completed etype similarity list $L$ which will be used for training the ML model or recognizing a candidate etype and entities. Notice that we present the algorithm for calculating the horizontal similarity $Sim_H$ in algorithm \ref{alg:1}, the metrics vertical similarity $Sim_V$ and informational similarity $Sim_I$ will be calculated by the same algorithm where the only modification is to change $HS_{KG}(\cdot)$ to $VS_{KG}(\cdot)$ and $IS_{KG}(\cdot)$, respectively. 

\subsection{Dataset EnType.}
We build the dataset EnType for validating the algorithm on instance-level etype recognition since there is no existing dataset for such a task released publicly. We exploit DBpedia infobox dataset\footnote{http://wikidata.dbpedia.org/services-resources/ontology} as the reference KG for providing reference etypes. Because DBpedia is a general-purpose KG that contains common etypes in the real world, where sufficient properties are applied for describing these etypes. Then we select candidate entities from DBpedia, SUMO\footnote{https://www.ontologyportal.org/} and several domain-specific datasets like Arnetminer dataset \cite{tang2008arnetminer}. 
The entities we selected mainly according to common etypes, more specifically, \textit{Person, Place, Event, Organization} and their sub-classes. Finally, we obtain 20,000 etype-entity candidate pairs for constructing two subsets EnType$_{Self}$ and EnType$_{Gen}$ which are distinguished by the resource of their candidate entities. 
Dataset EnType$_{Self}$ involves candidate pairs where reference etype and candidate entities are both selected from DBpedia\footnote{https://databus.dbpedia.org/dbpedia/mappings/instance-types/}. In turn, the candidate entities in EnType$_{Gen}$ are selected from the non-DBpedia resources. Both subsets are designed to simulate real-world instance-level etype recognition scenarios. The difficulty to solve  EnType$_{Self}$ is easier since the property matching performance will be better in this case. Need to notice that all datasets will be randomly separated into the training and testing sets to implement the corresponding ML model.

\subsection{Effect of constraint factor}
In the main manuscripts, we defined a constraint factor $\lambda$ for calculating the metric $Sim_H$. This study aims to statistically identify the value of $\lambda$. We apply the dataset ConfTrack and its two best-performed models. The value of $\lambda$ is set evenly from 0.1 to 1 by discrete points. We evaluate if this per-set factor affects the final recognition performance and obtain the best value of $\lambda$ for generic etype recognition. Table \ref{tab:7} demonstrates the results, where we highlight both the best and second-best results. We can find that different values of $\lambda$ do affect the final etype recognition performance. And two models show a similar trend that the best value of $\lambda$ is close to 0.5. As a result, we assign $\lambda = 0.5$ to calculate metric $Sim_H$ in our experiments.

\begin{table}[h]
\centering
\setlength{\abovecaptionskip}{5pt}    
\setlength{\belowcaptionskip}{2pt}
\caption{Ablation study on the constraint factor $\lambda$.The best and second-best results are highlighted in {\color[HTML]{FF0000} red} and {\color[HTML]{0070C0} blue}, respectively.}
\label{tab:7}
\resizebox{1\columnwidth}{!}{
\begin{tabular}{@{}clcccccccc@{}}
\toprule
\multicolumn{1}{c}{Factor} & \multicolumn{1}{c}{Model} & 0.2 & 0.3 & 0.4 & 0.5 & 0.6 & 0.7 & 0.8 & 0.9 \\ \midrule
\multirow{2}{*}{$\lambda$} & ETR$_{Sch}$-SGD  
& 0.650     & 0.644   & 0.681  & {\color[HTML]{FF0000} 0.706} & 0.685 & {\color[HTML]{0070C0} 0.698}  & 0.670  & 0.659 \\
\addlinespace & ETR$_{Sch}$-RF   
& 0.683     & 0.712    & 0.716   & {\color[HTML]{0070C0} 0.735} &  {\color[HTML]{FF0000} 0.739} & 0.720 & 0.699 & 0.707  \\ \bottomrule
\end{tabular}}
\end{table}
